# Supplementary material for: High-fidelity State Transfer Between Leaky Quantum Memories
Source: arXiv:2005.13062 ancillary file (2020-05-26)
Supplement: Supplementary file 1 [file QSTSupplemental2.pdf]

# Supplemental Material: Quantum State Transfer Between Memory Blocks

Eric Chatterjee, Matt Eichenfield, and Daniel Soh

February 21, 2020

## 0.1 Deriving the Coefficient Equations

We start with the general case of asymmetric blocks with differing rates of intermediate state extrinsic loss, i.e. $\kappa'_{ex} \neq \kappa_{ex}$. For the purpose of this analysis, we will define the dimensionless constant $\epsilon = \kappa'_{ex}/\kappa_{ex}$, which would reduce to 1 if the two blocks were identical. As discussed in the main text, we wish to keep the system in a dark superposition of the intermediate states $|10\rangle$ and $|01\rangle$ at all times, such that the wavepacket is never reflected from the second block. The following Lindbladian represents the loss due to wavepacket reflection:

$$\begin{aligned} L_{ex} &= \sqrt{\kappa_{ex}} a_1 + \sqrt{\kappa'_{ex}} a_2 \\ &= \sqrt{\kappa_{ex}} \Big( a_1 + \sqrt{\epsilon} a_2 \Big). \end{aligned} \tag{1}$$

The goal is for this Lindbladian to return a value of 0 when applied to the intermediate state part of the system wavefunction. To solve for this dark mode, we construct the following generic superposition of $a_1$ and $a_2$ modes:

$$|dark\rangle = c_1 |10\rangle + c_2 |01\rangle . \tag{2}$$

Applying the Lindbladian to this state and setting the output to 0, we derive the following equation relating $c_1$ and $c_2$:

$$c_1 + \sqrt{\epsilon} c_2 = 0. \tag{3}$$

The coefficients $c_1$ and $c_2$ must also satisfy the normalization condition:

$$(1 + \epsilon)|c_2|^2 = 1. \tag{4}$$

Solving the above 2 equations and substituting into Eq. (2), we find the dark mode wavefunction in terms of the two cavity modes:

$$|dark\rangle = \frac{1}{\sqrt{1+\epsilon}} \Big( |01\rangle - \sqrt{\epsilon} |10\rangle \Big). \tag{5}$$

In order to complete the photonic Hilbert subspace, it is also necessary to define the bright mode as orthogonal to the dark mode:

$$|bright\rangle = \frac{1}{\sqrt{1+\epsilon}}\Big(\sqrt{\epsilon}\,|01\rangle + |10\rangle\Big). \tag{6}$$

Next, we construct ladder operators corresponding to the new basis for the intermediate state Hilbert subspace, so that we can then re-write the Hamiltonian in terms of those operators. We denote the annihilation operator for a dark mode as follows:

$$a_d = |00\rangle\langle dark|\,. \tag{7}$$

Similarly, the annihilation operator for a bright mode is defined in the following manner:

$$a_b = |00\rangle\langle bright|\,. \tag{8}$$

From the dark and bright mode wavefunctions, we know that these ladder operators relate to $a_1$ and $a_2$ through the following system of equations:

$$a_d = \frac{1}{\sqrt{1+\epsilon}}\Big(a_2 - \sqrt{\epsilon}a_1\Big). \tag{9}$$

$$a_b = \frac{1}{\sqrt{1+\epsilon}}\Big(\sqrt{\epsilon}a_2 + a_1\Big). \tag{10}$$

We solve this system to find $a_1$ and $a_2$ in terms of $a_b$ and $a_d$:

$$a_1 = \frac{1}{\sqrt{1+\epsilon}}\Big(a_b - \sqrt{\epsilon}a_d\Big). \tag{11}$$

$$a_2 = \frac{1}{\sqrt{1+\epsilon}}\Big(\sqrt{\epsilon}a_b + a_d\Big). \tag{12}$$

We are now in a position to substitute these into the Hamiltonian. For equal rates of intrinsic loss, but unequal rates of extrinsic loss, the Hamiltonian takes the following form in terms of $a_1$ and $a_2$:

$$\begin{aligned} H_T^{eff} = &-\hbar g_1(t)(a_1^\dagger b_1 + a_1 b_1^\dagger) - \hbar g_2(t)(a_2^\dagger b_2 + a_2 b_2^\dagger) + \frac{i\hbar}{2}\sqrt{\kappa_{ex}\kappa'_{ex}}(a_1^\dagger a_2 - a_1 a_2^\dagger) \\ &- \frac{i\hbar}{2}(\sqrt{\kappa_{ex}}a_1^\dagger + \sqrt{\kappa'_{ex}}a_2^\dagger)(\sqrt{\kappa_{ex}}a_1 + \sqrt{\kappa'_{ex}}a_2) \\ &- i\hbar\frac{\kappa_i}{2}(a_1^\dagger a_1 + a_2^\dagger a_2) - i\hbar\frac{\Gamma_i}{2}(b_1^\dagger b_1 + b_2^\dagger b_2). \end{aligned} \tag{13}$$

Substituting Eq. (11) and (12) term-by-term:

$$a_1^\dagger b_1 + a_1 b_1^\dagger = \frac{1}{\sqrt{1+\epsilon}}\Big(a_b^\dagger b_1 - \sqrt{\epsilon} a_d^\dagger b_1 + a_b b_1^\dagger - \sqrt{\epsilon} a_d b_1^\dagger\Big). \tag{14}$$

$$a_2^\dagger b_2 + a_2 b_2^\dagger = \frac{1}{\sqrt{1+\epsilon}}\Big(\sqrt{\epsilon} a_b^\dagger b_2 + a_d^\dagger b_2 + \sqrt{\epsilon} a_b b_2^\dagger + a_d b_2^\dagger\Big). \tag{15}$$

$$\begin{aligned} a_1^\dagger a_2 - a_1 a_2^\dagger &= \frac{1}{1+\epsilon}\Big(a_b^\dagger a_d - a_b a_d^\dagger - \epsilon a_b a_d^\dagger + \epsilon a_b^\dagger a_d\Big) \\ &= \frac{1}{1+\epsilon}(1+\epsilon)(a_b^\dagger a_d - a_b a_d^\dagger) \\ &= a_b^\dagger a_d - a_b a_d^\dagger. \end{aligned} \tag{16}$$

From Eqs. (9) and (10):

$$\Big(a_1^\dagger + \sqrt{\epsilon} a_2^\dagger\Big)\Big(a_1 + \sqrt{\epsilon} a_2\Big) = (1+\epsilon) a_b^\dagger a_b. \tag{17}$$

Since the total intermediate state occupation number for bright and dark modes is the same as the total for the two cavity modes:

$$a_1^\dagger a_1 + a_2^\dagger a_2 = a_b^\dagger a_b + a_d^\dagger a_d. \tag{18}$$

These yield the following expression for the Hamiltonian in terms of the bright and dark state ladder operators:

$$\begin{aligned} H_T^{eff} = &\hbar g_1(t)\frac{\sqrt{\epsilon}}{\sqrt{1+\epsilon}}(a_d^\dagger b_1 + a_d b_1^\dagger) - \hbar g_1(t)\frac{1}{\sqrt{1+\epsilon}}(a_b^\dagger b_1 + a_b b_1^\dagger) \\ &- \hbar g_2(t)\frac{1}{\sqrt{1+\epsilon}}(a_d^\dagger b_2 + a_d b_2^\dagger) - \hbar g_2(t)\frac{\sqrt{\epsilon}}{\sqrt{1+\epsilon}}(a_b^\dagger b_2 + a_b b_2^\dagger) \\ &+ i\hbar\frac{\kappa_{ex}}{2}\sqrt{\epsilon}(a_b^\dagger a_d - a_b a_d^\dagger) - i\hbar\frac{\kappa_{ex}}{2}\frac{1}{1+\epsilon}a_b^\dagger a_b \\ &- i\hbar\frac{\kappa_i}{2}(a_b^\dagger a_b + a_d^\dagger a_d) - i\hbar\frac{\Gamma_i}{2}(b_1^\dagger b_1 + b_2^\dagger b_2). \end{aligned} \tag{19}$$

Since the system is always in a dark state, it is useful to consider only the matrix elements of the Hamiltonian corresponding to a dark initial state and thereby omit all

terms that annihilate the bright mode or return the bright mode occupation number:

$$\begin{aligned} H_T^{eff}\left|\Psi(t)\right\rangle\left\langle\Psi(t)\right| = &\hbar g_1(t)\frac{\sqrt{\epsilon}}{\sqrt{1+\epsilon}}(a_d^\dagger b_1 + a_d b_1^\dagger) - \hbar g_1(t)\frac{1}{\sqrt{1+\epsilon}}a_b^\dagger b_1 \\ &- \hbar g_2(t)\frac{1}{\sqrt{1+\epsilon}}(a_d^\dagger b_2 + a_d b_2^\dagger) - \hbar g_2(t)\frac{\sqrt{\epsilon}}{\sqrt{1+\epsilon}}a_b^\dagger b_2 \\ &+ i\hbar\frac{\kappa_{ex}}{2}\sqrt{\epsilon}a_b^\dagger a_d - i\hbar\frac{\kappa_i}{2}a_d^\dagger a_d - i\hbar\frac{\Gamma_i}{2}(b_1^\dagger b_1 + b_2^\dagger b_2). \end{aligned} \tag{20}$$

Importantly, the non-Hermitian term corresponding to loss due to wavepacket reflection, i.e. $-i\hbar\frac{\kappa_{ex}}{2}\frac{1}{1+\epsilon}a_b^\dagger a_b$, goes to 0 for the dark mode, thus validating our original method of rotating the basis for the photonic Hilbert subspace.

Next, we use the Schrodinger equation to establish a system of equations for the time-evolving state coefficients $\alpha_1(t)$, $\alpha_2(t)$, and $\beta_\alpha(t)$. Recall that the system wavefunction at any time $t$ can be expressed as follows:

$$\left|\Psi(t)\right\rangle = c_g\left|gg\right\rangle\left|00\right\rangle + c_e\Big(\alpha_1(t)\left|eg\right\rangle\left|00\right\rangle + \alpha_2(t)\left|ge\right\rangle\left|00\right\rangle + i\beta_\alpha(t)\left|gg\right\rangle\left|dark\right\rangle\Big). \tag{21}$$

Solving the matrix Schrodinger equation row-by-row, we obtain the following expressions:

$$\begin{aligned} i\hbar c_e\dot{\alpha_1}(t) &= \langle eg, 00|H_T^{eff}|\Psi(t)\rangle \\ &= c_e\Bigg(\hbar g_1(t)\frac{\sqrt{\epsilon}}{\sqrt{1+\epsilon}}(i\beta_\alpha(t)) - i\hbar\frac{\Gamma_i}{2}\alpha_1(t)\Bigg). \end{aligned} \tag{22}$$

$$\begin{aligned} i\hbar c_e\dot{\alpha_2}(t) &= \langle ge, 00|H_T^{eff}|\Psi(t)\rangle \\ &= c_e\Bigg(-\hbar g_2(t)\frac{1}{\sqrt{1+\epsilon}}(i\beta_\alpha(t)) - i\hbar\frac{\Gamma_i}{2}\alpha_2(t)\Bigg). \end{aligned} \tag{23}$$

$$\begin{aligned} -\hbar c_e\dot{\beta_\alpha}(t) &= \langle gg, dark|H_T^{eff}|\Psi(t)\rangle \\ &= c_e\Bigg(\hbar g_1(t)\frac{\sqrt{\epsilon}}{\sqrt{1+\epsilon}}\alpha_1(t) - \hbar g_2(t)\frac{1}{\sqrt{1+\epsilon}}\alpha_2(t) - i\hbar\frac{\kappa_i}{2}(i\beta_\alpha(t))\Bigg). \end{aligned} \tag{24}$$

It is also necessary for the coupling profiles to satisfy the following equation in order to prevent the Hamiltonian from coupling the dark mode into a bright mode:

$$\begin{aligned} 0 &= \langle gg, bright|H_T^{eff}|\Psi(t)\rangle \\ &= c_e\bigg( -\hbar g_1(t)\frac{1}{\sqrt{1+\epsilon}}\alpha_1(t) - \hbar g_2(t)\frac{\sqrt{\epsilon}}{\sqrt{1+\epsilon}}\alpha_2(t) + i\hbar\frac{\kappa_{ex}}{2}\sqrt{\epsilon}(i\beta_\alpha(t))\bigg). \end{aligned} \tag{25}$$

Dividing the first two equations by $i\hbar c_e$ and the latter two by $-\hbar c_e$, we find a system of differential equations for the time evolution of the coefficients:

$$\dot{\alpha_1}(t) = \frac{\sqrt{\epsilon}}{\sqrt{1+\epsilon}}g_1(t)\beta_\alpha(t) - \frac{\Gamma_i}{2}\alpha_1(t). \tag{26}$$

$$\dot{\alpha_2}(t) = -\frac{1}{\sqrt{1+\epsilon}}g_2(t)\beta_\alpha(t) - \frac{\Gamma_i}{2}\alpha_2(t). \tag{27}$$

$$\dot{\beta_\alpha}(t) = \frac{1}{\sqrt{1+\epsilon}}g_2(t)\alpha_2(t) - \frac{\sqrt{\epsilon}}{\sqrt{1+\epsilon}}g_1(t)\alpha_1(t) - \frac{\kappa_i}{2}\beta_\alpha(t). \tag{28}$$

$$0 = \frac{\sqrt{\epsilon}}{\sqrt{1+\epsilon}}g_2(t)\alpha_2(t) + \frac{1}{\sqrt{1+\epsilon}}g_1(t)\alpha_1(t) + \frac{\kappa_{ex}\sqrt{\epsilon}}{2}\beta_\alpha(t). \tag{29}$$

## 0.2 Solving for the Second Half of the Process

We will start by solving the coefficients for $t \geq 0$ (i.e. the second half of the transfer process), setting $g_1(t) = g_1(0)$ for this time range. Since the system in its final state has either fully entered the $b_2$ phonon mode $|ge\rangle|00\rangle$ or has collapsed to the vacuum state $|gg\rangle|00\rangle$, $\alpha_1(t)$ and $\beta_\alpha(t)$ will converge to 0 as $t \to \infty$ and we therefore start by solving for those coefficients. The coupling profile $g_2(t)$ can be determined in terms of the state coefficients and the constant $g_1(0)$ by re-arranging Eq. (29) as follows:

$$\begin{aligned} g_2(t) &= -\frac{\sqrt{1+\epsilon}}{\sqrt{\epsilon}}\frac{\left(\frac{\kappa_{ex}\sqrt{\epsilon}}{2}\beta_\alpha(t) + \frac{1}{\sqrt{1+\epsilon}}g_1(0)\alpha_1(t)\right)}{\alpha_2(t)} \\ &= -\frac{\left(\frac{\kappa_{ex}\sqrt{1+\epsilon}}{2}\beta_\alpha(t) + \frac{1}{\sqrt{\epsilon}}g_1(0)\alpha_1(t)\right)}{\alpha_2(t)}. \end{aligned} \tag{30}$$

Substituting this into Eq. (28), we find the following expression for $\dot{\beta}_\alpha(t)$ in terms of $\alpha_1(t)$ and $\beta_\alpha(t)$:

$$\begin{aligned}\dot{\beta}_\alpha(t) &= \frac{1}{\sqrt{1+\epsilon}}\left(-\frac{\kappa_{ex}\sqrt{1+\epsilon}}{2}\beta_\alpha(t) - \frac{1}{\sqrt{\epsilon}}g_1(0)\alpha_1(t)\right) - \frac{\sqrt{\epsilon}}{\sqrt{1+\epsilon}}g_1(0)\alpha_1(t) - \frac{\kappa_i}{2}\beta_\alpha(t) \\ &= -\frac{1}{\sqrt{1+\epsilon}}\left(\frac{1}{\sqrt{\epsilon}} + \sqrt{\epsilon}\right)g_1(0)\alpha_1(t) - \frac{\kappa_{ex}+\kappa_i}{2}\beta_\alpha(t) \\ &= -\frac{\sqrt{1+\epsilon}}{\sqrt{\epsilon}}g_1(0)\alpha_1(t) - \frac{\kappa_{ex}+\kappa_i}{2}\beta_\alpha(t).\end{aligned} \tag{31}$$

Combining Eqs. (26) and (31), we express the resulting system of differential equations as a matrix ODE:

$$\begin{pmatrix}\dot{\alpha_1}(t) \\ \dot{\beta}_\alpha(t)\end{pmatrix} = \begin{pmatrix}-\frac{\Gamma_i}{2} & \frac{\sqrt{\epsilon}}{\sqrt{1+\epsilon}}g_1(0) \\ -\frac{\sqrt{1+\epsilon}}{\sqrt{\epsilon}} & -\frac{\kappa_{ex}+\kappa_i}{2}\end{pmatrix}\begin{pmatrix}\alpha_1(t) \\ \beta_\alpha(t)\end{pmatrix}. \tag{32}$$

The eigenvalues turn out to be independent of $\epsilon$:

$$\lambda_\pm = -\frac{1}{4}(\Gamma_i + \kappa_{ex} + \kappa_i) \pm \frac{C}{4}. \tag{33}$$

Here, $C = \sqrt{(\Gamma_i - \kappa_{ex} - \kappa_i)^2 - 16g_1(0)^2}$. The corresponding eigenvectors, on the other hand, vary with $\epsilon$ in the following manner:

$$v_\pm = \begin{pmatrix}(\Gamma_i - \kappa_{ex} - \kappa_i \mp C)\sqrt{\epsilon} \\ 4g_1(0)\sqrt{1+\epsilon}\end{pmatrix}. \tag{34}$$

Recall that the solutions for a matrix ODE are functions of the eigenvalues, eigenvectors, and constants that are to be determined from the boundary values:

$$\begin{pmatrix}\alpha_1(t) \\ \beta_\alpha(t)\end{pmatrix} = Ae^{\lambda_- t}v_- + Be^{\lambda_+ t}v_+. \tag{35}$$

It is worth noting that since the eigenvalues are independent of $\epsilon$, the time-dependence of the individual terms in the solution will also be invariant in $\epsilon$. Instead, only the

constant coefficient in each term will change. This is evident from expressing the solutions in the following form:

$$\begin{pmatrix}\alpha_1(t)\\ \beta_\alpha(t)\end{pmatrix} = e^{-\frac{1}{4}(\Gamma_i+\kappa_{ex}+\kappa_i)t}\Big(Ae^{-\frac{C}{4}t}v_- + Be^{\frac{C}{4}t}v_+\Big)$$
$$= e^{-\frac{1}{4}(\Gamma_i+\kappa_{ex}+\kappa_i)t}\bigg(\Big(Av_- + Bv_+\Big)\cosh\left(\frac{C}{4}t\right) + \bigg(\Big(Bv_+ - Av_-\Big)\sinh\left(\frac{C}{4}t\right)\bigg). \tag{36}$$

The generic matrix ODE solution leads to the following system of equations for $\alpha_1(0)$ and $\beta_\alpha(0)$ in terms of $A$ and $B$:

$$\alpha_1(0) = \Big((\Gamma_i - \kappa_{ex} - \kappa_i + C)A + (\Gamma_i - \kappa_{ex} - \kappa_i - C)B\Big)\sqrt{\epsilon}. \tag{37}$$

$$\beta_\alpha(0) = 4g_1(0)\sqrt{1+\epsilon}(A+B). \tag{38}$$

Solving this system of equations, we find the following expressions for $A$ and $B$:

$$A = \frac{1}{2C}\bigg(\frac{1}{\sqrt{\epsilon}}\alpha_1(0) - \frac{\Gamma_i - \kappa_{ex} - \kappa_i - C}{4g_1(0)\sqrt{1+\epsilon}}\beta_\alpha(0)\bigg). \tag{39}$$

$$B = \frac{1}{2C}\bigg(-\frac{1}{\sqrt{\epsilon}}\alpha_1(0) + \frac{\Gamma_i - \kappa_{ex} - \kappa_i + C}{4g_1(0)\sqrt{1+\epsilon}}\beta_\alpha(0)\bigg). \tag{40}$$

We first focus on solving $\alpha_1(t)$ by subsituting $A$, $B$, $v_{-,1}$, and $v_{+,1}$ into the constant coefficient expressions in Eq. (36):

$$\begin{aligned} Av_{-,1} + Bv_{+,1} &= \frac{1}{2C}\bigg(\frac{1}{\sqrt{\epsilon}}\alpha_1(0) - \frac{\Gamma_i - \kappa_{ex} - \kappa_i - C}{4g_1(0)\sqrt{1+\epsilon}}\beta_\alpha(0)\bigg)(\Gamma_i - \kappa_{ex} - \kappa_i + C)\sqrt{\epsilon} \\ &\quad + \frac{1}{2C}\bigg(\frac{-1}{\sqrt{\epsilon}}\alpha_1(0) + \frac{\Gamma_i - \kappa_{ex} - \kappa_i + C}{4g_1(0)\sqrt{1+\epsilon}}\beta_\alpha(0)\bigg)(\Gamma_i - \kappa_{ex} - \kappa_i - C)\sqrt{\epsilon} \\ &= \frac{1}{2C}\bigg(\frac{2}{\sqrt{\epsilon}}\alpha_1(0)C\sqrt{\epsilon}\bigg) \\ &= \alpha_1(0). \end{aligned} \tag{41}$$

$$
\begin{aligned}
Bv_{+,1} - Av_{-,1} &= \frac{1}{2C}\left(\frac{-1}{\sqrt{\epsilon}}\alpha_1(0) + \frac{\Gamma_i - \kappa_{ex} - \kappa_i + C}{4g_1(0)\sqrt{1+\epsilon}}\beta_\alpha(0)\right)(\Gamma_i - \kappa_{ex} - \kappa_i - C)\sqrt{\epsilon} \\
&\quad - \frac{1}{2C}\left(\frac{1}{\sqrt{\epsilon}}\alpha_1(0) - \frac{\Gamma_i - \kappa_{ex} - \kappa_i - C}{4g_1(0)\sqrt{1+\epsilon}}\beta_\alpha(0)\right)(\Gamma_i - \kappa_{ex} - \kappa_i + C)\sqrt{\epsilon} \\
&= \frac{1}{2C}\left( -2(\Gamma_i - \kappa_{ex} - \kappa_i)\alpha_1(0) + \frac{(\Gamma_i - \kappa_{ex} - \kappa_i)^2 - C^2}{2g_1(0)}\frac{\sqrt{\epsilon}}{\sqrt{1+\epsilon}}\beta_\alpha(0)\right) \\
&= \frac{1}{2C}\left(2(\kappa_{ex} + \kappa_i - \Gamma_i)\alpha_1(0) + \frac{16g_1(0)^2}{2g_1(0)}\frac{\sqrt{\epsilon}}{\sqrt{1+\epsilon}}\beta_\alpha(0)\right) \\
&= \frac{1}{C}\left((\kappa_{ex} + \kappa_i - \Gamma_i)\alpha_1(0) + 4g_1(0)\sqrt{\frac{\epsilon}{1+\epsilon}}\beta_\alpha(0)\right).
\end{aligned}
\tag{42}
$$

Subsituting these into Eq. (36), we find the following expression for $\alpha_1(t)$ for $t \geq 0$:

$$
\begin{aligned}
\alpha_1(t) &= e^{-\frac{1}{4}(\Gamma_i + \kappa_{ex} + \kappa_i)t}\left(\left(Av_{-,1} + Bv_{+,1}\right)\cosh\left(\frac{C}{4}t\right) + \left(\left(Bv_{+,1} - Av_{-,1}\right)\sinh\left(\frac{C}{4}t\right)\right)\right. \\
&= \frac{e^{-\frac{1}{4}(\kappa_{ex} + \kappa_i + \Gamma_i)t}}{C}\left(\alpha_1(0)C\cosh\left(\frac{C}{4}t\right)\right. \\
&\quad \left. + \left(4\sqrt{\frac{\epsilon}{1+\epsilon}}g_1(0)\beta_\alpha(0) + \alpha_1(0)(\kappa_{ex} + \kappa_i - \Gamma_i)\right)\sinh\left(\frac{C}{4}t\right)\right).
\end{aligned}
\tag{43}
$$

Note that only the coefficient in the second term in this expression varies with $\epsilon$. When $\epsilon = 1$, that coefficient reduces to $2\sqrt{2}g_1(0)\beta_\alpha(0)$.

We now complete an analogous set of steps to determine $\beta_\alpha(t)$. Subsituting $A$, $B$, $v_{-,2}$, and $v_{+,2}$ into the constant coefficient expressions in Eq. (36):

$$
\begin{aligned}
Av_{-,2} + Bv_{+,2} &= \frac{1}{2C}\left(\frac{1}{\sqrt{\epsilon}}\alpha_1(0) - \frac{\Gamma_i - \kappa_{ex} - \kappa_i - C}{4g_1(0)\sqrt{1+\epsilon}}\beta_\alpha(0)\right)4g_1(0)\sqrt{1+\epsilon} \\
&\quad + \frac{1}{2C}\left(\frac{-1}{\sqrt{\epsilon}}\alpha_1(0) + \frac{\Gamma_i - \kappa_{ex} - \kappa_i + C}{4g_1(0)\sqrt{1+\epsilon}}\beta_\alpha(0)\right)4g_1(0)\sqrt{1+\epsilon} \\
&= \frac{1}{2C}\left(\frac{2C}{4g_1(0)\sqrt{1+\epsilon}}\beta_\alpha(0)\right)4g_1(0)\sqrt{1+\epsilon} \\
&= \beta_\alpha(0).
\end{aligned}
\tag{44}
$$

$$
\begin{aligned}
Bv_{+,2} - Av_{-,2} &= \frac{1}{2C}\left(\frac{-1}{\sqrt{\epsilon}}\alpha_1(0) + \frac{\Gamma_i - \kappa_{ex} - \kappa_i + C}{4g_1(0)\sqrt{1+\epsilon}}\beta_\alpha(0)\right)4g_1(0)\sqrt{1+\epsilon} \\
&\quad - \frac{1}{2C}\left(\frac{1}{\sqrt{\epsilon}}\alpha_1(0) - \frac{\Gamma_i - \kappa_{ex} - \kappa_i - C}{4g_1(0)\sqrt{1+\epsilon}}\beta_\alpha(0)\right)4g_1(0)\sqrt{1+\epsilon} \\
&= \frac{1}{2C}\left(\frac{-2}{\sqrt{\epsilon}}\alpha_1(0) + \frac{\Gamma_i - \kappa_{ex} - \kappa_i}{2g_1(0)\sqrt{1+\epsilon}}\beta_\alpha(0)\right)4g_1(0)\sqrt{1+\epsilon} \\
&= -\frac{1}{C}\left(4\sqrt{\frac{1+\epsilon}{\epsilon}}g_1(0)\alpha_1(0) + \beta_\alpha(0)(\kappa_{ex} + \kappa_i - \Gamma_i)\right).
\end{aligned}
\tag{45}
$$

We substitute these into Eq. (36) to find $\beta_\alpha(t)$ for $t \geq 0$ as follows:

$$
\begin{aligned}
\beta_\alpha(t) &= e^{-\frac{1}{4}(\Gamma_i+\kappa_{ex}+\kappa_i)t}\left(\left(Av_{-,2} + Bv_{+,2}\right)\cosh\left(\frac{C}{4}t\right) + \left(\left(Bv_{+,2} - Av_{-,2}\right)\sinh\left(\frac{C}{4}t\right)\right)\right. \\
&= \frac{e^{-\frac{1}{4}(\kappa_{ex}+\kappa_i+\Gamma_i)t}}{C}\left(\beta_\alpha(0)C\cosh\left(\frac{C}{4}t\right)\right. \\
&\quad \left. - \left(4\sqrt{\frac{1+\epsilon}{\epsilon}}g_1(0)\alpha_1(0) + \beta_\alpha(0)(\kappa_{ex} + \kappa_i - \Gamma_i)\right)\sinh\left(\frac{C}{4}t\right)\right).
\end{aligned}
\tag{46}
$$

Note that only the second term (i.e. the first term in the paranthesis) varies with $\epsilon$. When $\epsilon = 1$, the coefficient in that term reduces to $4\sqrt{2}g_1(0)\alpha_1(0)$.

We finally undertake the process of solving for $\alpha_2(t)$. Substituting the expression for $g_2(t)$ from Eq. (30) into that for $\dot{\alpha_2}(t)$ from Eq. (27), we find the following differential equation:

$$
\begin{aligned}
\dot{\alpha_2}(t) &= -\frac{1}{\sqrt{1+\epsilon}}\frac{\left(-\frac{\kappa_{ex}\sqrt{1+\epsilon}}{2}\beta_\alpha(t) - \frac{1}{\sqrt{\epsilon}}g_1(0)\alpha_1(t)\right)}{\alpha_2(t)}\beta_\alpha(t) - \frac{\Gamma_i}{2}\alpha_2(t) \\
&= \frac{\left(\frac{\kappa_{ex}}{2}\beta_\alpha(t) + \frac{g_1(0)}{\sqrt{\epsilon(1+\epsilon)}}\alpha_1(t)\right)}{\alpha_2(t)}\beta_\alpha(t) - \frac{\Gamma_i}{2}\alpha_2(t).
\end{aligned}
\tag{47}
$$

Multiplying both sides by $2\alpha_2(t)$, the expression becomes a first-order ordinary differential equation in $\alpha_2^2$:

$$
\begin{aligned}
\frac{d}{dt}\alpha_2(t)^2 &= 2\alpha_2(t)\dot{\alpha_2}(t) \\
&= \left(\kappa_{ex}\beta_\alpha(t)^2 + \frac{2g_1(0)}{\sqrt{\epsilon(1+\epsilon)}}\alpha_1(t)\beta_\alpha(t)\right) - \Gamma_i\alpha_2^2(t).
\end{aligned}
\tag{48}
$$

Note that the time-varying part of each of the constituent terms is invariant in $\epsilon$. We integrate the equation term-by-term:

$$\alpha_2(t)^2 = e^{-\Gamma_i t}\left(\kappa_{ex}\int e^{\Gamma_i t}\beta_\alpha(t)^2 dt + \frac{2g_1(0)}{\sqrt{\epsilon(1+\epsilon)}}\int e^{\Gamma_i t}\alpha_1(t)\beta_\alpha(t)dt + G\right). \tag{49}$$

Here, $G$ is a constant that will eventually be calculated from the boundary conditions for $\alpha_2(t)^2$. For now, we focus on the first term inside the paranthesis. Our first goal is to examine $\int e^{\Gamma_i t}\beta_\alpha(t)^2 dt$. The integrand can be expanded by substituting the expression for $\beta_\alpha(t)$ from Eq. (46):

$$\begin{aligned} e^{\Gamma_i t}\beta_\alpha(t)^2 = \frac{e^{-\frac{1}{2}(\kappa_{ex}+\kappa_i-\Gamma_i)t}}{C^2}\Bigg(&\beta_\alpha(0)^2 C^2\cosh^2\left(\frac{C}{4}t\right) \\ &- 2B_1'\beta_\alpha(0)C\cosh\left(\frac{C}{4}t\right)\sinh\left(\frac{C}{4}t\right) + B_1'^2\sinh^2\left(\frac{C}{4}t\right)\Bigg). \end{aligned} \tag{50}$$

For each of the terms in Eq. (50), we integrate the time-dependent part using Mathematica and then multiply by the associated constant. For the first term, we find the following result:

$$\begin{aligned} &\beta_\alpha(0)^2\int e^{-\frac{1}{2}(\kappa_{ex}+\kappa_i-\Gamma_i)t}\cosh^2\left(\frac{C}{4}t\right) \\ &= \frac{\beta_\alpha(0)^2 e^{\frac{1}{2}(\Gamma_i-\kappa_{ex}-\kappa_i)t}}{(\Gamma_i-\kappa_{ex}-\kappa_i)((\Gamma_i-\kappa_{ex}-\kappa_i)^2-C^2)}\Bigg(-C^2 - C(\Gamma_i-\kappa_{ex}-\kappa_i)\sinh\left(\frac{C}{2}t\right) \\ &\quad + (\Gamma_i-\kappa_{ex}-\kappa_i)^2\cosh^2\left(\frac{C}{2}t\right) + (\Gamma_i-\kappa_{ex}-\kappa_i)^2\Bigg). \end{aligned} \tag{51}$$

For the second term, we find the following:

$$\begin{aligned} &-\frac{2B_1'\beta_\alpha(0)}{C}\int e^{-\frac{1}{2}(\kappa_{ex}+\kappa_i-\Gamma_i)t}\cosh\left(\frac{C}{4}t\right)\sinh\left(\frac{C}{4}t\right) \\ &= \frac{2B_1'\beta_\alpha(0)e^{\frac{1}{2}(\Gamma_i-\kappa_{ex}-\kappa_i)t}}{C((\Gamma_i-\kappa_{ex}-\kappa_i)^2-C^2)}\left((\kappa_{ex}+\kappa_i-\Gamma_i)\sinh\left(\frac{C}{2}t\right) + C\cosh\left(\frac{C}{2}t\right)\right). \end{aligned} \tag{52}$$

Finally, the third term yields the following:

$$\frac{B_1'^2}{C^2}\int e^{-\frac{1}{2}(\kappa_{ex}+\kappa_i-\Gamma_i)t}\sinh^2\left(\frac{C}{4}t\right)$$
$$=\frac{B_1'^2 e^{\frac{1}{2}(\Gamma_i-\kappa_{ex}-\kappa_i)t}}{C^2(\Gamma_i-\kappa_{ex}-\kappa_i)((\Gamma_i-\kappa_{ex}-\kappa_i)^2-C^2)}\Bigg(C^2-C(\Gamma_i-\kappa_{ex}-\kappa_i)\sinh\left(\frac{C}{2}t\right)$$
$$+(\Gamma_i-\kappa_{ex}-\kappa_i)^2\cosh^2\left(\frac{C}{2}t\right)-(\Gamma_i-\kappa_{ex}-\kappa_i)^2\Bigg). \tag{53}$$

Note that all 3 of these expressions contain the term $(\Gamma_i-\kappa_{ex}-\kappa_i)^2-C^2$ in the denominator, which simply equals $16g_1(0)^2$. Summing the 3 expressions, we find the following result for $\int e^{\Gamma_i t}\beta_\alpha(t)^2 dt$:

$$\int e^{\Gamma_i t}\beta_\alpha(t)^2 dt=\frac{e^{\frac{1}{2}(\Gamma_i-\kappa_{ex}-\kappa_i)t}}{16g_1(0)^2}\Big(\beta_\alpha(0)^2A_1(t)+2B_1'\beta_\alpha(0)A_2(t)+B_1'^2A_3(t)\Big). \tag{54}$$

where we have defined $A_1(t)$, $A_2(t)$, and $A_3(t)$ as follows:

$$A_1(t)=\frac{-C^2-C(\Gamma_i-\kappa_i-\kappa_{ex})\sinh\left(\frac{C}{2}t\right)+(\Gamma_i-\kappa_i-\kappa_{ex})^2\Big(\cosh\left(\frac{C}{2}t\right)+1\Big)}{\Gamma_i-\kappa_i-\kappa_{ex}}. \tag{55}$$

$$A_2(t)=\frac{-(\Gamma_i-\kappa_i-\kappa_{ex})\sinh\left(\frac{C}{2}t\right)+C\cosh\left(\frac{C}{2}t\right)}{C}. \tag{56}$$

$$A_3(t)=\frac{C^2-C(\Gamma_i-\kappa_i-\kappa_{ex})\sinh\left(\frac{C}{2}t\right)+(\Gamma_i-\kappa_i-\kappa_{ex})^2\Big(\cosh\left(\frac{C}{2}t\right)-1\Big)}{C^2(\Gamma_i-\kappa_i-\kappa_{ex})}. \tag{57}$$

Next, we examine $\int e^{\Gamma_i t}\alpha_1(t)\beta_\alpha(t)dt$. We expand the integrand in a manner analogous to Eq. (50), this time by substituting $\alpha_1(t)$ from Eq. (43) and $\beta_\alpha(t)$ from Eq. (46):

$$e^{\Gamma_i t}\alpha_1(t)\beta_\alpha(t)=\frac{e^{-\frac{1}{2}(\kappa_{ex}+\kappa_i-\Gamma_i)t}}{C^2}\Bigg(\alpha_1(0)\beta_\alpha(0)C^2\cosh^2\left(\frac{C}{4}t\right)$$
$$-\Big(\alpha_1(0)B_1'-\beta_\alpha(0)B_2'\Big)C\cosh\left(\frac{C}{4}t\right)\sinh\left(\frac{C}{4}t\right) \tag{58}$$
$$+(-B_1'B_2')\sinh^2\left(\frac{C}{4}t\right)\Bigg).$$

Analyzing Eq. (58), we observe that the form of the expression is equivalent to that for $e^{\Gamma_i t}\beta_\alpha(t)^2$ in Eq. (50), with the replacements $\beta_\alpha(0)^2 \to \alpha_1(0)\beta_\alpha(0)$ in the first term, $2B_1'\beta_\alpha(0) \to \alpha_1(0)B_1' - \beta_\alpha(0)B_2'$ in the second term, and $B_1'^2 \to -B_1'B_2'$ in the third term. We therefore determine $\int e^{\Gamma_i t}\alpha_1(t)\beta_\alpha(t)dt$ simply by using Eq. (54) and implementing these replacements:

$$\begin{aligned}\int e^{\Gamma_i t}\alpha_1(t)\beta_\alpha(t)dt = \frac{e^{\frac{1}{2}(\Gamma_i-\kappa_{ex}-\kappa_i)t}}{16g_1(0)^2}\Big(&\alpha_1(0)\beta_\alpha(0)A_1(t) + \Big(\alpha_1(0)B_1' - \beta_\alpha(0)B_2'\Big)A_2(t)\\ &- B_1'B_2'A_3(t)\Big).\end{aligned} \tag{59}$$

Superposing these integrals using the coefficients in Eq. (49), we find the following result for $\alpha_2(t)^2$ for $t \geq 0$:

$$\begin{aligned}\alpha_2(t)^2 &= e^{-\Gamma_i t}\left(\kappa_{ex}\int e^{\Gamma_i t}\beta_\alpha(t)^2dt + \frac{2g_1(0)}{\sqrt{\epsilon(1+\epsilon)}}\int e^{\Gamma_i t}\alpha_1(t)\beta_\alpha(t)dt + G\right)\\ &= \frac{e^{-\frac{1}{2}(\kappa_{ex}+\kappa_i+\Gamma_i)t}}{16g_1(0)^2}\left(\left(\kappa_{ex}\beta_\alpha(0)^2 + \frac{2g_1(0)}{\sqrt{\epsilon(1+\epsilon)}}\alpha_1(0)\beta_\alpha(0)\right)A_1(t)\right.\\ &\quad + \left(2\kappa_{ex}B_1'\beta_\alpha(0) + \frac{2g_1(0)}{\sqrt{\epsilon(1+\epsilon)}}\Big(\alpha_1(0)B_1' - \beta_\alpha(0)B_2'\Big)\right)A_2(t)\\ &\quad \left. + \left(\kappa_{ex}B_1'^2 - \frac{2g_1(0)}{\sqrt{\epsilon(1+\epsilon)}}B_1'B_2'\right)A_3(t)\right) + Ge^{-\Gamma_i t}.\end{aligned} \tag{60}$$

Regarding the term $Ge^{-\Gamma_i t}$, it is useful to note that $\Gamma_i \ll \kappa_{ex}, \kappa_{ex}', \kappa_i$. Therefore, given the timescale of the transfer process, $e^{-\Gamma_i t}$ will approximately equal 1. Since the first term in the $\alpha_2(t)^2$ expression converges to 0 as $t \to t_f$, $G$ will approximately equal $\alpha_2^2(t_f)$, representing the fidelity of states for the process.

## 0.3 Solving for the First Half of the Process

We now analyze the time range $t < 0$, representing the first half of the process. Here, $g_2(t) = g_2(0)$ will be constant in time, whereas $g_1(t)$ will be variable. Since the system

is fully in the $b_1$ mode initially, we know that $\alpha_2(t)$ and $\beta_\alpha(t)$ will converge to 0 for the maximally negative value of $t$. As such, we start by solving for the time-evolution of those coefficients. Re-arranging Eq. (29) yields the following expression for $g_1(t)$ in terms of $g_2(0)$ and the state coefficients:

$$\begin{aligned} g_1(t) &= -\sqrt{1+\epsilon}\frac{\left(\frac{\kappa_{ex}\sqrt{\epsilon}}{2}\beta_\alpha(t) + \frac{\sqrt{\epsilon}}{\sqrt{1+\epsilon}}g_2(0)\alpha_2(t)\right)}{\alpha_1(t)} \\ &= -\frac{\left(\frac{\kappa_{ex}\sqrt{\epsilon(1+\epsilon)}}{2}\beta_\alpha(t) + \sqrt{\epsilon}g_2(0)\alpha_2(t)\right)}{\alpha_1(t)}. \end{aligned} \tag{61}$$

Substituting this into Eq. (28), we find a modified differential equation for $\dot{\beta_\alpha}(t)$ in terms of $\alpha_2(t)$ and $\beta_\alpha(t)$:

$$\begin{aligned} \dot{\beta_\alpha}(t) &= \frac{1}{\sqrt{1+\epsilon}}g_2(0)\alpha_2(t) - \frac{\sqrt{\epsilon}}{\sqrt{1+\epsilon}}\left(-\frac{\kappa_{ex}\sqrt{\epsilon(1+\epsilon)}}{2}\beta_\alpha(t) - \sqrt{\epsilon}g_2(0)\alpha_2(t)\right) \\ &\quad - \frac{\kappa_i}{2}\beta_\alpha(t) \\ &= \frac{1}{\sqrt{1+\epsilon}}(1+\epsilon)g_2(0)\alpha_2(t) - \frac{\kappa_i - \epsilon\kappa_{ex}}{2}\beta_\alpha(t) \\ &= \sqrt{1+\epsilon}g_2(0)\alpha_2(t) - \frac{\kappa_i - \epsilon\kappa_{ex}}{2}\beta_\alpha(t). \end{aligned} \tag{62}$$

The matrix ODE for $\dot{\alpha_2}(t)$ and $\dot{\beta_\alpha}(t)$ thus takes the following form:

$$\begin{pmatrix} \dot{\alpha_2}(t) \\ \dot{\beta_\alpha}(t) \end{pmatrix} = \begin{pmatrix} -\frac{\Gamma_i}{2} & -\frac{1}{\sqrt{1+\epsilon}}g_2(0) \\ \sqrt{1+\epsilon}g_2(0) & -\frac{\kappa_{ex}-\epsilon\kappa_i}{2} \end{pmatrix} \begin{pmatrix} \alpha_2(t) \\ \beta_\alpha(t) \end{pmatrix}. \tag{63}$$

The eigenvalues are similar to those for $t > 0$, except for the replacements $\kappa_{ex} \to -\epsilon\kappa_{ex}$ and $g_1(0)^2 \to g_2(0)^2$. As such, they can be expressed in terms of a constant $D'$ instead of $D$:

$$\lambda_{pm} = -\frac{1}{4}(\Gamma_i - \epsilon\kappa_{ex} + \kappa_i) \pm \frac{D'}{4}. \tag{64}$$

where $D'$ is defined as follows:

$$D' = \sqrt{(\Gamma_i + \epsilon\kappa_{ex} - \kappa_i)^2 - 16g_2(0)^2}. \tag{65}$$

The corresponding eigenvectors vary with $\epsilon$ in the following manner:

$$v_{\pm} = \begin{pmatrix} \Gamma_i + \epsilon\kappa_{ex} - \kappa_i \mp D' \\ -4g_2(0)\sqrt{1+\epsilon} \end{pmatrix}. \tag{66}$$

Recall that the solution set for $\alpha_2(t)$ and $\beta_\alpha(t)$ takes the following generic form:

$$\begin{pmatrix} \alpha_2(t) \\ \beta_\alpha(t) \end{pmatrix} = Ae^{\lambda_- t}v_- + Be^{\lambda_+ t}v_+. \tag{67}$$

Since the change in the eigenvalues from the $t > 0$ case is fully mediated through the replacements $\kappa_{ex} \to -\epsilon\kappa_{ex}$ and $C \to D'$, the time-variance of the individual terms in the solution can also be determined by simply modifying the $t > 0$ case by applying the aforementioned replacements, as evidenced by expressing the equations in the following form:

$$\begin{aligned} \begin{pmatrix} \alpha_2(t) \\ \beta_\alpha(t) \end{pmatrix} &= e^{-\frac{1}{4}(\Gamma_i - \epsilon\kappa_{ex} + \kappa_i)t}\Big(Ae^{-\frac{D'}{4}t}v_- + Be^{\frac{D'}{4}t}v_+\Big) \\ &= e^{-\frac{1}{4}(\Gamma_i - \epsilon\kappa_{ex} + \kappa_i)t}\left(\Big(Av_- + Bv_+\Big)\cosh\left(\frac{D'}{4}t\right)\right. \\ &\quad \left. + \left(\Big(Bv_+ - Av_-\Big)\sinh\left(\frac{D'}{4}t\right)\right)\right). \end{aligned} \tag{68}$$

We now aim to solve the constants $A$ and $B$. The generic matrix ODE solution yields the following system of equations for $\alpha_2(0)$ and $\beta_\alpha(0)$ in terms of these constants:

$$\alpha_2(0) = (\Gamma_i + \epsilon\kappa_{ex} - \kappa_i + D')A + (\Gamma_i + \epsilon\kappa_{ex} - \kappa_i - D')B. \tag{69}$$

$$\beta_\alpha(0) = -4g_2(0)\sqrt{1+\epsilon}(A+B). \tag{70}$$

From this system of equations, we find the following expressions for $A$ and $B$:

$$A = \frac{1}{2D'}\left(\alpha_2(0) + \frac{\Gamma_i + \epsilon\kappa_{ex} - \kappa_i - D'}{4g_2(0)\sqrt{1+\epsilon}}\beta_\alpha(0)\right). \tag{71}$$

$$B = -\frac{1}{2D'}\left(\alpha_2(0) + \frac{\Gamma_i + \epsilon\kappa_{ex} - \kappa_i + D'}{4g_2(0)\sqrt{1+\epsilon}}\beta_\alpha(0)\right). \tag{72}$$

Next, we use the values of $A$, $B$, $v_{+,1}$, and $v_{-,1}$ to calculate the constant coefficients in Eq. (68) for $\alpha_2(t)$. Starting with the coefficient in front of $\cosh\left(D't/4\right)$:

$$\begin{aligned}
Av_{-,1} + Bv_{+,1} &= \frac{1}{2D'}\left(\alpha_2(0) + \frac{\Gamma_i + \epsilon\kappa_{ex} - \kappa_i - D'}{4g_2(0)\sqrt{1+\epsilon}}\beta_\alpha(0)\right)(\Gamma_i + \epsilon\kappa_{ex} - \kappa_i + D') \\
&\quad - \frac{1}{2D'}\left(\alpha_2(0) + \frac{\Gamma_i + \epsilon\kappa_{ex} - \kappa_i + D'}{4g_2(0)\sqrt{1+\epsilon}}\beta_\alpha(0)\right)(\Gamma_i + \epsilon\kappa_{ex} - \kappa_i - D') \\
&= \frac{1}{2D'}\Big(2D'\alpha_2(0)\Big) \\
&= \alpha_2(0).
\end{aligned} \tag{73}$$

For the coefficient in front of $\sinh\left(D't/4\right)$:

$$\begin{aligned}
Bv_{+,1} - Av_{-,1} &= -\frac{1}{2D'}\left(\alpha_2(0) + \frac{\Gamma_i + \epsilon\kappa_{ex} - \kappa_i + D'}{4g_2(0)\sqrt{1+\epsilon}}\beta_\alpha(0)\right)(\Gamma_i + \epsilon\kappa_{ex} - \kappa_i - D') \\
&\quad - \frac{1}{2D'}\left(\alpha_2(0) + \frac{\Gamma_i + \epsilon\kappa_{ex} - \kappa_i - D'}{4g_2(0)\sqrt{1+\epsilon}}\beta_\alpha(0)\right)(\Gamma_i + \epsilon\kappa_{ex} - \kappa_i + D') \\
&= -\frac{1}{2D'}\left(2(\Gamma_i + \epsilon\kappa_{ex} - \kappa_i)\alpha_2(0) + \frac{(\Gamma_i + \epsilon\kappa_{ex} - \kappa_i)^2 - D'^2}{2g_2(0)\sqrt{1+\epsilon}}\beta_\alpha(0)\right) \\
&= -\frac{1}{2D'}\left(2(\Gamma_i + \epsilon\kappa_{ex} - \kappa_i)\alpha_2(0) + \frac{16g_2(0)^2}{2g_2(0)\sqrt{1+\epsilon}}\beta_\alpha(0)\right) \\
&= \frac{1}{D'}\left((\kappa_i - \epsilon\kappa_{ex} - \Gamma_i)\alpha_2(0) - \frac{4g_2(0)}{\sqrt{1+\epsilon}}\beta_\alpha(0)\right).
\end{aligned} \tag{74}$$

We substitute these into Eq. (68) to find $\alpha_2(t)$ for $t \leq 0$:

$$\begin{aligned}
\alpha_2(t) = \frac{e^{\frac{1}{4}(\epsilon\kappa_{ex} - \kappa_i - \Gamma_i)t}}{D'}&\left(\alpha_2(0)D'\cosh\left(\frac{D'}{4}t\right)\right. \\
&\left. + \left(-\frac{4g_2(0)}{\sqrt{1+\epsilon}}\beta_\alpha(0) + \alpha_2(0)(-\epsilon\kappa_{ex} + \kappa_i - \Gamma_i)\right)\sinh\left(\frac{D'}{4}t\right)\right).
\end{aligned} \tag{75}$$

Note that the constant coefficient in the second term (i.e. the first term in the paranthesis) reduces to $-2\sqrt{2}g_2(0)\beta_\alpha(0)$ if $\epsilon = 1$.

We now look to solve $\beta_\alpha(t)$, starting by subsituting the values of $A$, $B$, $v_{+,2}$, and $v_{-,2}$ to determine the second-row constant coefficients in Eq. (68). Starting with the

coefficient associated with $\cosh(D't/4)$:

$$
\begin{aligned}
Av_{-,2} + Bv_{+,2} &= \frac{1}{2D'}\left(\alpha_2(0) + \frac{\Gamma_i + \epsilon\kappa_{ex} - \kappa_i - D'}{4g_2(0)\sqrt{1+\epsilon}}\beta_\alpha(0)\right)\left(-4g_2(0)\sqrt{1+\epsilon}\right) \\
&\quad - \frac{1}{2D'}\left(\alpha_2(0) + \frac{\Gamma_i + \epsilon\kappa_{ex} - \kappa_i + D'}{4g_2(0)\sqrt{1+\epsilon}}\beta_\alpha(0)\right)\left(-4g_2(0)\sqrt{1+\epsilon}\right) \\
&= \frac{1}{2D'}\left(\frac{-2D'}{4g_2(0)\sqrt{1+\epsilon}}\beta_\alpha(0)\right)\left(-4g_2(0)\sqrt{1+\epsilon}\right) \\
&= \beta_\alpha(0).
\end{aligned}
\tag{76}
$$

For the coefficient associated with $\sinh(D't/4)$:

$$
\begin{aligned}
Bv_{+,2} - Av_{-,2} &= -\frac{1}{2D'}\left(\alpha_2(0) + \frac{\Gamma_i + \epsilon\kappa_{ex} - \kappa_i + D'}{4g_2(0)\sqrt{1+\epsilon}}\beta_\alpha(0)\right)\left(-4g_2(0)\sqrt{1+\epsilon}\right) \\
&\quad - \frac{1}{2D'}\left(\alpha_2(0) + \frac{\Gamma_i + \epsilon\kappa_{ex} - \kappa_i - D'}{4g_2(0)\sqrt{1+\epsilon}}\beta_\alpha(0)\right)\left(-4g_2(0)\sqrt{1+\epsilon}\right) \\
&= -\frac{1}{2D'}\left(2\alpha_2(0) + \frac{\Gamma_i + \epsilon\kappa_{ex} - \kappa_i}{2g_2(0)\sqrt{1+\epsilon}}\beta_\alpha(0)\right)\left(-4g_2(0)\sqrt{1+\epsilon}\right) \\
&= -\frac{1}{D'}\Big(-4\Big(\sqrt{1+\epsilon}\Big)g_2(0)\alpha_2(0) + (\kappa_i - \epsilon\kappa_{ex} - \Gamma_i)\beta_\alpha(0)\Big).
\end{aligned}
\tag{77}
$$

Substituting these into Eq. (68), we find $\beta_\alpha(t)$ for $t \le 0$:

$$
\begin{aligned}
\beta_\alpha(t) = \frac{e^{\frac{1}{4}(\epsilon\kappa_{ex} - \kappa_i - \Gamma_i)t}}{D'}\Bigg(&\beta_\alpha(0)D'\cosh\left(\frac{D'}{4}t\right) \\
&- \Big(-4\Big(\sqrt{1+\epsilon}\Big)g_2(0)\alpha_2(0) + \beta_\alpha(0)(-\epsilon\kappa_{ex} + \kappa_i - \Gamma_i)\Big)\sinh\left(\frac{D'}{4}t\right)\Bigg).
\end{aligned}
\tag{78}
$$

If $\epsilon = 1$, the first term in the paranthesis reduces to $-4\sqrt{2}g_2(0)\alpha_2(0)$.

Finally, we work to solve $\alpha_1(t)$ for the first half of the process. Substituting the expression for $g_1(t)$ from Eq. (61) into that for $\dot{\alpha_1}(t)$ from Eq. (26), we obtain the

following differential equation:

$$\begin{aligned}\dot{\alpha_1}(t) &= \frac{\sqrt{\epsilon}}{\sqrt{1+\epsilon}} \frac{\Big(-\frac{\kappa_{ex}\sqrt{\epsilon(1+\epsilon)}}{2}\beta_\alpha(t) - \sqrt{\epsilon}g_2(0)\alpha_2(t)\Big)}{\alpha_1(t)}\beta_\alpha(t) - \frac{\Gamma_i}{2}\alpha_1(t) \\ &= \frac{\Big(-\frac{\kappa_{ex}\epsilon}{2}\beta_\alpha(t) - \frac{\epsilon}{\sqrt{1+\epsilon}}g_2(0)\alpha_2(t)\Big)}{\alpha_1(t)}\beta_\alpha(t) - \frac{\Gamma_i}{2}\alpha_1(t).\end{aligned} \tag{79}$$

Multiplying both sides by $2\alpha_1(t)$, the expression becomes a first-order ordinary differential equation in $\alpha_1^2$:

$$\begin{aligned}\frac{d}{dt}\alpha_1(t)^2 &= 2\alpha_1(t)\dot{\alpha_1}(t) \\ &= \Big(-\kappa_{ex}\epsilon\beta_\alpha(t)^2 - \frac{2\epsilon}{\sqrt{1+\epsilon}}g_2(0)\alpha_2(t)\beta_\alpha(t)\Big) - \Gamma_i\alpha_1(t)^2.\end{aligned} \tag{80}$$

As with the other first-order ODE that we have solved, we integrate this equation term-by-term:

$$\alpha_1(t)^2 = e^{-\Gamma_i t}\Big(-\kappa_{ex}\epsilon\int e^{\Gamma_i t}\beta_\alpha(t)^2 dt - \frac{2\epsilon}{\sqrt{1+\epsilon}}g_2(0)\int e^{\Gamma_i t}\alpha_2(t)\beta_\alpha(t)dt + G'\Big). \tag{81}$$

We observe that $\alpha_2(t)$ and $\beta_\alpha(t)$ for $t \leq 0$ are identical to $\alpha_1(t)$ and $\beta_\alpha(t)$ (respectively) for $t \geq 0$ upon making the replacements $C \to D'$, $\kappa_{ex} \to -\epsilon\kappa_{ex}$, $\alpha_1(0) \to \alpha_2(0)$, $B_1' \to B_3'$, and $B_2' \to B_4'$, where $B_3'$ and $B_4'$ represent the paranthetical expressions in the solutions $\beta_\alpha(t)$ and $\alpha_2(t)$, respectively:

$$B_3' = -4\Big(\sqrt{1+\epsilon}\Big)g_2(0)\alpha_2(0) + \beta_\alpha(0)(-\epsilon\kappa_{ex} + \kappa_i - \Gamma_i). \tag{82}$$

$$B_4' = -\frac{4g_2(0)}{\sqrt{1+\epsilon}}\beta_\alpha(0) + \alpha_2(0)(-\epsilon\kappa_{ex} + \kappa_i - \Gamma_i). \tag{83}$$

We apply the relevant replacements to solve for $\int e^{\Gamma_i t}\beta_\alpha(t)^2 dt$ and $\int e^{\Gamma_i t}\alpha_2(t)\beta_\alpha(t)dt$ based on the analogous results for $t \geq 0$ from Eqs. (54) and (59):

$$\int e^{\Gamma_i t}\beta_\alpha(t)^2 dt = \frac{e^{\frac{1}{2}(\Gamma_i + \epsilon\kappa_{ex} - \kappa_i)t}}{16g_2(0)^2}\Big(\beta_\alpha(0)^2 A_4'(t) + 2B_3'\beta_\alpha(0)A_5'(t) + B_3'^2 A_6'(t)\Big). \tag{84}$$

$$\int e^{\Gamma_i t}\alpha_1(t)\beta_\alpha(t)dt = \frac{e^{\frac{1}{2}(\Gamma_i+\epsilon\kappa_{ex}-\kappa_i)t}}{16g_2(0)^2}\Big(\alpha_2(0)\beta_\alpha(0)A_4'(t) + \Big(\alpha_2(0)B_3' - \beta_\alpha(0)B_4'\Big)A_5'(t) - B_3'B_4'A_6(t)\Big). \tag{85}$$

where $A_4'(t)$, $A_5'(t)$, and $A_6'(t)$ are defined by applying the relevant replacements to $A_1(t)$, $A_2(t)$, and $A_3(t)$, respectively:

$$A_4'(t) = \frac{-D'^2 - D'(\Gamma_i - \kappa_i + \epsilon\kappa_{ex})\sinh\left(\frac{D'}{2}t\right) + (\Gamma_i - \kappa_i + \epsilon\kappa_{ex})^2\Big(\cosh\left(\frac{D'}{2}t\right) + 1\Big)}{\Gamma_i - \kappa_i + \epsilon\kappa_{ex}}. \tag{86}$$

$$A_5'(t) = \frac{-(\Gamma_i - \kappa_i + \epsilon\kappa_{ex})\sinh\left(\frac{D'}{2}t\right) + D'\cosh\left(\frac{D'}{2}t\right)}{D'}. \tag{87}$$

$$A_6'(t) = \frac{D'^2 - D'(\Gamma_i - \kappa_i + \epsilon\kappa_{ex})\sinh\left(\frac{D'}{2}t\right) + (\Gamma_i - \kappa_i + \epsilon\kappa_{ex})^2\Big(\cosh\left(\frac{D'}{2}t\right) - 1\Big)}{D'^2(\Gamma_i - \kappa_i + \epsilon\kappa_{ex})}. \tag{88}$$

Substituting the above 2 integrals into Eq. (81), we find the following expression for $\alpha_1(t)^2$ for $t \leq 0$:

$$\begin{aligned}
\alpha_1(t)^2 &= e^{-\Gamma_i t}\Big( - \kappa_{ex}\epsilon\int e^{\Gamma_i t}\beta_\alpha(t)^2 dt - \frac{2\epsilon}{\sqrt{1+\epsilon}}\int e^{\Gamma_i t}\alpha_1(t)\beta_\alpha(t)dt + G'\Big) \\
&= \frac{e^{-\frac{1}{2}(-\epsilon\kappa_{ex}+\kappa_i+\Gamma_i)t}}{16g_2(0)^2}\Bigg(\Big( - \kappa_{ex}\epsilon\beta_\alpha(0)^2 - \frac{2\epsilon}{\sqrt{1+\epsilon}}g_2(0)\alpha_2(0)\beta_\alpha(0)\Big)A_4'(t) \\
&\quad + \Big( - 2\kappa_{ex}\epsilon B_3'\beta_\alpha(0) - \frac{2\epsilon}{\sqrt{1+\epsilon}}g_2(0)\Big(\alpha_2(0)B_3' - \beta_\alpha(0)B_4'\Big)\Big)A_5'(t) \\
&\quad + \Big( - \kappa_{ex}\epsilon B_3'^2 + \frac{2\epsilon}{\sqrt{1+\epsilon}}g_2(0)B_3'B_4'\Big)A_6(t)\Bigg) + G'e^{-\Gamma_i t}.
\end{aligned} \tag{89}$$

Since the system is initially in the $b_1$ mode, and since $e^{-\Gamma_i t} \approx 1$ for the timescale of the transfer process, $G'$ will equal 1.

## 0.4 Computational Methods

Having found solutions for the time-evolution of the coefficients $\alpha_1(t)$, $\alpha_2(t)$, and $\beta_\alpha(t)$ in terms of their values at $t = 0$, our next task is to calculate the range of possible zero-point values the corresponding coupling profiles $g_1(t)$ and $g_2(t)$. To this end, we use MATLAB-based computation, setting pre-determined values for $g_1(0)$ and $g_2(0)$. Starting by looping over all possible values of $\alpha_2(0)$ and $\beta_\alpha(0)$, we substitute these into Eq. (89) to determine $\alpha_1(0)$ for every pair of the input zero-point coefficients. To ensure the validity of the resulting coefficient trios, we only keep the results that closely match the condition in Eq. (29). Finally, we loop over the filtered list of zero-point coefficient trios and substitute them into Eq. (60) to determine the fidelity $\alpha_2(t_f)^2$ for each trio. With the resulting knowledge of the time evolution of the coefficients, it is straightforward to use Eq. (29) to derive $g_1(t)$ for $t < 0$ and $g_2(t)$ for $t > 0$. The results demonstrate that the fidelity is invariant in the choices of $g_1(0)$ and $g_2(0)$, while varying specifically with the ratio of intrinsic loss rate to output coupling rate for each of the blocks.
